# Supplementary material for: Universal relations for hybridized $s$- and $p$-wave interactions from spin-orbital coupling
Source: arXiv:2005.04997 source file (2020-10-20)
Supplement: Supplementary file 1 [file 1dsocmix_supp_20200627.pdf]

# Supplemental Material

Fang Qin (覃昉)[1,2] and Pengfei Zhang[3,4,*]

[1] Shenzhen Institute for Quantum Science and Engineering and Department of Physics, Southern University of Science and Technology (SUSTech), Shenzhen 518055, China

[2] CAS Key Laboratory of Quantum Information, University of Science and Technology of China, Chinese Academy of Sciences, Hefei, Anhui 230026, China

[3] Walter Burke Institute for Theoretical Physics, California Institute of Technology, Pasadena, California 91125, USA

[4] Institute for Quantum Information and Matter, California Institute of Technology, Pasadena, California 91125, USA

(Dated: October 20, 2020)

In this Supplemental Material, we provide the detailed calculations for the results in the main text.

## CONTENTS

SI. Model S1

SII. Dimer propagator matrix S3

SIII. Contact matrix S5

SIV. Momentum tail S5

SV. Raman spectroscopy S6

SVI. Other universal relations S7
- A. Adiabatic relations S7
- B. Pressure relation S7
- C. Virial theorem S8

SVII. Contacts in two-body bound states S9

SVIII. Appendix S10
- A. Derivations of Eq. (S10) S10
- B. Derivations of Eq. (S28) S12
- C. Derivations of Eq. (S33) S13
- D. $T$ matrix for $s$ wave without SOC S13
- E. $T$ matrix for $p$ wave without SOC S14

References S14

## SI. MODEL

The effective 1D Lagrangian with SOC is given by ($\hbar = 1$ throughout the paper)

$$\hat{L} = \sum_{k,\sigma=\uparrow,\downarrow} \psi^\dagger_{k,\sigma}\left(i\partial_t - \frac{k^2}{2m}\right)\psi_{k,\sigma} - \Omega\sum_k\left(e^{i2k_0x}\psi^\dagger_{k,\uparrow}\psi_{k,\downarrow} + e^{-i2k_0x}\psi^\dagger_{k,\downarrow}\psi_{k,\uparrow}\right)$$
$$-\frac{g_S}{L}\sum_{Q,k,k'}\psi^\dagger_{Q/2-k',\downarrow}\psi^\dagger_{Q/2+k',\uparrow}\psi_{Q/2+k,\uparrow}\psi_{Q/2-k,\downarrow} - \frac{g_P}{4L}\sum_{Q,k,k'}k'\psi^\dagger_{Q/2-k',\uparrow}\psi^\dagger_{Q/2+k',\uparrow}k\psi_{Q/2+k,\uparrow}\psi_{Q/2-k,\uparrow}, \quad \text{(S1)}$$

* pengfeizhang.physics@gmail.com

where $\psi_{k,\sigma}$ is the field operator for the fermionic atoms in terms of the momentum $k$ and $g_S$ ($g_P/4$) is the effective 1D $s(p)$-wave coupling constant. The Fermi atoms in the state $|\uparrow\rangle$ are coupled to the state $|\downarrow\rangle$ by the Raman laser with the strength $\Omega = \Omega_R/2$, $\Omega_R$ is the Rabi frequency, $2k_0$ is the momentum transfer during the two-photon processes, and $L$ is the system size. Here, we have included the $s$-wave interaction between atoms with spin $\uparrow$ and $\downarrow$, together with a $p$-wave interaction between two spin-$\uparrow$ fermions.

The interaction part of the Lagrangian in the momentum space can be changed into

$$\hat{L}_{\text{int}} = -\frac{1}{\sqrt{L}}\sum_{Q,k}\left(\varphi^{\dagger}_{Q,S}\psi_{Q/2+k,\uparrow}\psi_{Q/2-k,\downarrow} + \text{H.c.}\right) - \frac{1}{2\sqrt{L}}\sum_{Q,k} k\left(\varphi^{\dagger}_{Q,P}\psi_{Q/2+k,\uparrow}\psi_{Q/2-k,\uparrow} + \text{H.c.}\right) + \sum_{Q;\alpha=S,P}\frac{\varphi^{\dagger}_{Q,\alpha}\varphi_{Q,\alpha}}{g_\alpha}, \tag{S2}$$

where we use the definitions $\varphi^{\dagger}_{Q,S} \equiv g_S\sum_{k'}\psi^{\dagger}_{Q/2-k',\downarrow}\psi^{\dagger}_{Q/2+k',\uparrow}/\sqrt{L}$, $\varphi^{\dagger}_{Q,P} \equiv \frac{1}{2}g_P\sum_{k'}k'\psi^{\dagger}_{Q/2-k',\uparrow}\psi^{\dagger}_{Q/2+k',\uparrow}/\sqrt{L}$, and $\varphi_{Q,S}$ ($\varphi_{Q,P}$) is the field operator of the $s(p)$-wave dimer.

With the definitions of $\varphi^{\dagger}_{Q,S}$ and $\varphi^{\dagger}_{Q,P}$, the derivations of the last term in Eq. (S2) are as follows:

$$\sum_{Q;\alpha=S,P}\frac{\varphi^{\dagger}_{Q,\alpha}\varphi_{Q,\alpha}}{g_\alpha} = \frac{g_S}{L}\sum_{Q,k,k'}\psi^{\dagger}_{Q/2-k',\downarrow}\psi^{\dagger}_{Q/2+k',\uparrow}\psi_{Q/2+k,\uparrow}\psi_{Q/2-k,\downarrow} + \frac{g_P}{4L}\sum_{Q,k,k'}k'\psi^{\dagger}_{Q/2-k',\uparrow}\psi^{\dagger}_{Q/2+k',\uparrow}k\psi_{Q/2+k,\uparrow}\psi_{Q/2-k,\uparrow}. \tag{S3}$$

Generally, the SOC couples $s$-wave and $p$-wave dimers, and we would show that we do not need to introduce $\varphi^{\dagger}_{Q,S}\varphi_{Q,P}/g_{SP}$ to regularize the possible divergence.

To remove the phase factor $e^{\pm i2k_0x}$ in the second term of Eq. (S1), we introduce two new atomic fields: $\psi_{k,\uparrow} = \psi_{k,\uparrow}e^{ik_0x}$ and $\psi_{k,\downarrow} = \psi_{k,\downarrow}e^{-ik_0x}$. Then, we can write the single-particle part of the Hamiltonian in the momentum space: $H_0 = \sum_k \Psi^{\dagger}_k\mathcal{H}^0_k\Psi_k$ with $\Psi_k = (\psi_{k,\uparrow}, \psi_{k,\downarrow})^T$ and

$$\mathcal{H}^0_k = \begin{pmatrix} \frac{(k+k_0)^2}{2m} & \Omega \\ \Omega & \frac{(k-k_0)^2}{2m} \end{pmatrix}. \tag{S4}$$

Therefore, the inverse of the single-particle propagator matrix is given by [1, 2]

$$G^{-1}(\omega,k) = -i\begin{pmatrix} \omega + i0^+ - \frac{(k+k_0)^2}{2m} & -\Omega \\ -\Omega & \omega + i0^+ - \frac{(k-k_0)^2}{2m} \end{pmatrix}. \tag{S5}$$

To calculate the Feynman diagrams for simplicity, the Lagrangian can be written into

$$\hat{L} = \sum_k \Psi^{\dagger}_k\left(i\partial_t - \mathcal{H}^0_k\right)\Psi_k + \sum_{Q;\alpha=S,P}\frac{\varphi^{\dagger}_{Q,\alpha}\varphi_{Q,\alpha}}{g_\alpha} - \frac{1}{\sqrt{L}}\sum_{Q,k}\left[\varphi^{\dagger}_{Q,S}\left(\frac{1}{2}\Psi^T_{Q/2+k}S\Psi_{Q/2-k}\right) + \text{H.c.}\right] - \frac{1}{2\sqrt{L}}\sum_{Q,k}k\left[\varphi^{\dagger}_{Q,P}\left(\Psi^T_{Q/2+k}P\Psi_{Q/2-k}\right) + \text{H.c.}\right], \tag{S6}$$

where $\sigma_S = i\sigma_y$, $\sigma_P = \frac{1}{2}(1+\sigma_z)$, $\sigma_j$ ($j = x, y, z$) is the Pauli matrix, and we have

$$\frac{1}{2}\Psi^T_{Q/2+k}\sigma_S\Psi_{Q/2-k} = \psi_{Q/2+k,\uparrow}\psi_{Q/2-k,\downarrow}, \tag{S7}$$

$$\Psi^T_{Q/2+k}\sigma_P\Psi_{Q/2-k} = \psi_{Q/2+k,\uparrow}\psi_{Q/2-k,\uparrow}. \tag{S8}$$

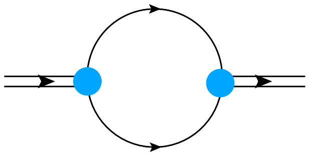

FIG. S1. Feynman diagrams for the matrix elements of the dimer-atom interaction operator. The single line denotes the bare atom propagator matrix $G$, the double lines denote the matrix elements of the dimer propagator martrix $D_{\alpha\beta}$ with $\alpha, \beta \in \{S, P\}$, and the blue dot represents the interaction vertex: $-i\sigma_\alpha$ or $-i\sigma_\beta$.

## SII. DIMER PROPAGATOR MATRIX

We consider finite total momentum $Q$ for each two-body pairing state. As shown in Fig. S1, the inverse of the dimer propagator matrix is given by the Dyson equation

$$\begin{aligned} D^{-1}(E_0,Q) &= \begin{pmatrix} (ig_S)^{-1} & 0 \\ 0 & (ig_P)^{-1} \end{pmatrix} - \begin{pmatrix} \Pi_{SS}(E_0,Q) & \Pi_{SP}(E_0,Q) \\ \Pi_{PS}(E_0,Q) & \Pi_{PP}(E_0,Q) \end{pmatrix} \\ &= \begin{pmatrix} (ig_S)^{-1} - \Pi_{SS}(E_0,Q) & -\Pi_{SP}(E_0,Q) \\ -\Pi_{PS}(E_0,Q) & (ig_P)^{-1} - \Pi_{PP}(E_0,Q) \end{pmatrix}, \end{aligned} \tag{S9}$$

where the polarization bubble is given by (the derivations are given in the Appendix)

$$\Pi_{\alpha\beta}(E_0,Q) = -\int \frac{dpdp_0}{(2\pi)^2} \frac{p^{l_\alpha + l_\beta}}{2} \mathrm{Tr}\left[ G^T(p_0, Q/2+p)\sigma_\alpha G(E_0 - p_0, Q/2 - p)\sigma_\beta^\dagger \right], \tag{S10}$$

$E_0 = Q^2/(4m) + k^2/m$ is the total energy, $\alpha, \beta \in \{S, P\}$, $l_S = 0$, $l_P = 1$, and Tr denotes the trace over the spin degrees of freedom.

For convenience, one can also write the dimer propagator matrix as

$$D(E_0,Q) = \frac{1}{\det[D^{-1}(E_0,Q)]} \begin{pmatrix} (ig_P)^{-1} - \Pi_{PP}(E_0,Q) & \Pi_{SP}(E_0,Q) \\ \Pi_{PS}(E_0,Q) & (ig_S)^{-1} - \Pi_{SS}(E_0,Q) \end{pmatrix} = \begin{pmatrix} D_{SS}(E_0,Q) & D_{SP}(E_0,Q) \\ D_{PS}(E_0,Q) & D_{PP}(E_0,Q) \end{pmatrix}, \tag{S11}$$

where $\det[D^{-1}(E_0,Q)]$ is the determinant of $D^{-1}(E_0,Q)$.

In the absence of the Raman coupling, the $s$-wave polarization bubble is given by

$$\Pi_{SS}(E_0,Q) = -\int \frac{dpdp_0}{(2\pi)^2} \frac{i}{p_0 - (Q/2+p)^2/(2m) + i0^+} \frac{i}{E_0 - p_0 - (Q/2-p)^2/(2m) + i0^+} = -\frac{m}{2k}, \tag{S12}$$

where we use $E_0 = Q^2/(4m) + k^2/m$.

The 1D scattering amplitude can be written as [3, 4] $f_{1D}(k) = -1/(1 + i\cot\delta_k) \simeq -1/(1 + ika_s)$, where $\delta_k$ is the scattering phase shift. With the $s$-wave $T$ matrix $T_s(k) = ikf_{1D}(k)/m_r$ and $D_{SS}(k) = iT_s(k)$, one can get

$$a_s = -\frac{2}{mg_S}, \tag{S13}$$

where $a_s$ is the effective 1D $s$-wave scattering length.

In the absence of the Raman coupling, the $p$-wave polarization bubble is given by

$$\begin{aligned} \Pi_{PP}(E_0,Q) &= -\frac{1}{2}\int \frac{dpdp_0}{(2\pi)^2} \frac{ip^2}{p_0 - (Q/2+p)^2/(2m) + i0^+} \frac{i}{E_0 - p_0 - (Q/2-p)^2/(2m) + i0^+} \\ &= -\frac{1}{2}\int \frac{dp}{2\pi} \frac{ip^2}{E_0 - Q^2/(4m) - p^2/m + i0^+} = \frac{im}{2}\int_{-\Lambda}^{\Lambda} \frac{dp}{2\pi} \frac{(p^2 - k^2) + k^2}{[p - (k + i0^+)][p + (k + i0^+)]} \\ &= \frac{im}{2}\left(\frac{\Lambda}{\pi} + i\frac{k}{2}\right), \end{aligned} \tag{S14}$$

where $\Lambda$ is the ultraviolet momentum cutoff and we use $E_0 = Q^2/(4m) + k^2/m$.

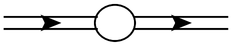

FIG. S2. Feynman diagrams for the matrix elements of the dimer local operator $\varphi_\alpha^\dagger(R)\varphi_\beta(R)$ and its derivatives $\varphi_\alpha^\dagger(R)\left[i\partial_t+\partial_R^2/(4m)\right]^u(-i\partial_R)^v\varphi_\beta(R)$ with $u,v=0,1,2,3,\cdots$. The open dot represents the operators.

Therefore, the $p$-wave $T$ matrix is given by

$$\frac{T_{pp}(E_0,Q)}{qq'}=\frac{D_{PP}(E_0,Q)}{i}=\frac{1}{\frac{1}{g_P}-i\Pi_{pp}(E_0,Q)}=\frac{1}{\frac{1}{g_P}+\frac{m\Lambda}{2\pi}+i\frac{mk}{4}}. \tag{S15}$$

Comparing Eq. (S15) with [5]

$$\frac{T_{pp}(E_0,Q)}{qq'}=\frac{1}{\frac{m}{4a_p}+i\frac{mk}{4}}, \tag{S16}$$

one can get

$$\frac{m}{4a_p}=\frac{1}{g_P}+\frac{m\Lambda}{2\pi}, \tag{S17}$$

where $a_p$ is the effective 1D $p$-wave scattering length.

In the presence of the Raman fields, the bubble with zero total momentum ($Q=0$) can be calculated as

$$\begin{aligned}\Pi_{SS}(E_0,0)=&\frac{-m^3\Omega^2}{2(mE_0k_0^2-k_0^4+m^2\Omega^2)\sqrt{mE_0+i0^+-k_0^2}}-\frac{mk_0^2}{4}\left[\frac{\sqrt{mE_0+k_0^2+2\sqrt{mE_0k_0^2+m^2\Omega^2}}}{m^2\Omega^2+k_0^2(mE_0+\sqrt{mE_0k_0^2+m^2\Omega^2})}\right.\\&\left.+\frac{\sqrt{mE_0+i0^++k_0^2-2\sqrt{mE_0k_0^2+m^2\Omega^2}}}{m^2\Omega^2+k_0^2(mE_0-\sqrt{mE_0k_0^2+m^2\Omega^2})}\right]\approx\frac{-m}{2\sqrt{mE_0}},\end{aligned} \tag{S18}$$

$$\begin{aligned}\Pi_{PP}(E_0,0)=&\frac{im}{2}\left(\frac{\Lambda}{\pi}+i\frac{\sqrt{mE_0+i0^+-k_0^2}}{2}\right)-\frac{m^3\Omega^2}{16}\left(\frac{\sqrt{mE_0+k_0^2+2\sqrt{mE_0k_0^2+m^2\Omega^2}}}{mE_0k_0^2+m^2\Omega^2+k_0^2\sqrt{mE_0k_0^2+m^2\Omega^2}}\right.\\&\left.+\frac{\sqrt{mE_0+i0^++k_0^2-2\sqrt{mE_0k_0^2+m^2\Omega^2}}}{mE_0k_0^2+m^2\Omega^2-k_0^2\sqrt{mE_0k_0^2+m^2\Omega^2}}\right)\approx\frac{im}{2}\left(\frac{\Lambda}{\pi}+i\frac{\sqrt{mE_0+i0^+-k_0^2}}{2}\right),\end{aligned} \tag{S19}$$

$$\begin{aligned}\Pi_{SP}(E_0,0)=&\,\Pi_{PS}(E_0,0)\\=&\frac{m^2k_0\Omega\sqrt{mE_0+i0^+-k_0^2}}{4(mE_0k_0^2-k_0^4+m^2\Omega^2)}-\frac{m^2k_0\Omega}{8}\left(\frac{\sqrt{mE_0+k_0^2+2\sqrt{mE_0k_0^2+m^2\Omega^2}}}{mE_0k_0^2+m^2\Omega^2+k_0^2\sqrt{mE_0k_0^2+m^2\Omega^2}}\right.\\&\left.+\frac{\sqrt{mE_0+i0^++k_0^2-2\sqrt{mE_0k_0^2+m^2\Omega^2}}}{mE_0k_0^2+m^2\Omega^2-k_0^2\sqrt{mE_0k_0^2+m^2\Omega^2}}\right)\approx\frac{\sqrt{m}k_0\Omega}{8E_0^{-3/2}},\end{aligned} \tag{S20}$$

where $k_0$ and $\Omega$ are treated perturbatively up to the $k_0^2$ and $\Omega$ order. Note that Eq. (S17) can be used to cancel the divergence of the $p$-wave bubble (S19), and the $s$- and $p$-wave mixing bubble (S20) needs both finite $k_0$ and $\Omega$, as expected from having a non-trivial SOC.

In the absence of the Raman coupling, the quasi-1D $s(p)$-wave scattering length connected to the three-dimensional (3D) one is given by [6–14]

$$a_s=-\frac{\ell_\perp^2}{2a_{3D}}+\frac{\mathcal{C}\ell_\perp}{2}, \tag{S21}$$

$$a_p=\frac{3V_p}{\ell_\perp^2}, \tag{S22}$$

where $a_{3D}$ is the 3D $s$-wave scattering length, $\mathcal{C}=1.4603$, $\ell_\perp=\sqrt{2/(m\omega_\perp)}$, $\omega_\perp$ is the transverse trapping frequency, and $V_p$ is the 3D $p$-wave scattering volume.

## SIII. CONTACT MATRIX

For simplicity to define the contact matrix, the Lagrangian (S1) can be transformed into the coordinate $R$ space:

$$\hat{L} = \sum_{\sigma=\uparrow,\downarrow} \int dR\, \psi_\sigma^\dagger \left( i\partial_t + \frac{\partial_R^2}{2m} \right) \psi_\sigma - \Omega \int dR\, \left( e^{i2k_0R} \psi_\uparrow^\dagger \psi_\downarrow + e^{-i2k_0R} \psi_\downarrow^\dagger \psi_\uparrow \right) + \sum_{\alpha=S,P} \int dR \frac{\varphi_\alpha^\dagger \varphi_\alpha}{g_\alpha}$$
$$- \int dR \left( \varphi_S^\dagger \psi_\uparrow \psi_\downarrow + \text{H.c.} \right) - \frac{1}{2} \int dR\, \left\{ \varphi_P^\dagger \left[ (-i\partial_R \psi_\uparrow)\psi_\uparrow - \psi_\uparrow(-i\partial_R \psi_\uparrow) \right] + \text{H.c.} \right\}, \tag{S23}$$

where $\psi_\sigma$ is the field operator for the fermionic atoms in terms of the time $t$ and the coordinate $R$, and $\varphi_S$ ($\varphi_P$) is the field operator of the $s(p)$-wave dimer also in terms of the time $t$ and the coordinate $R$.

The contact operator matrix can be defined in terms of the field operators as

$$\frac{\hat{C}_{\alpha\beta}^{(u,v)}(R)}{m^{2+u}} = \varphi_\alpha^\dagger(R) \left( i\partial_t + \frac{\partial_R^2}{4m} \right)^u (-i\partial_R)^v \varphi_\beta(R)$$
$$= \begin{pmatrix} \varphi_S^\dagger(R) \left( i\partial_t + \frac{\partial_R^2}{4m} \right)^u (-i\partial_R)^v \varphi_S(R) & \varphi_S^\dagger(R) \left( i\partial_t + \frac{\partial_R^2}{4m} \right)^u (-i\partial_R)^v \varphi_P(R) \\ \varphi_P^\dagger(R) \left( i\partial_t + \frac{\partial_R^2}{4m} \right)^u (-i\partial_R)^v \varphi_S(R) & \varphi_P^\dagger(R) \left( i\partial_t + \frac{\partial_R^2}{4m} \right)^u (-i\partial_R)^v \varphi_S(R) \end{pmatrix}_{\alpha\beta}, \tag{S24}$$

where $u, v = 0, 1, 2, 3, \cdots$.

To compute the momentum tail, instead of incoming and outgoing states with a pair of fermions, we consider a single incoming dimer $|I_{\alpha_i}\rangle = \int dtdR\, e^{i(E_0 t - QR)} \varphi_{\alpha_i}^\dagger(R,t) |0\rangle$ and a single outgoing dimer $\langle O_{\alpha_o}| = \int dtdR\, e^{-i(E_0 t - QR)} \langle 0| \varphi_{\alpha_o}(R,t)$. Therefore, as shown in Fig. S2, the matrix elements of the contact matrix are given by:

$$\frac{C_{\alpha\beta}^{(u,v)}}{m^{2+u}} = \int dR\, \langle O_{\alpha_o}| \varphi_\alpha^\dagger(R,t) \left( i\partial_t + \frac{\partial_R^2}{4m} \right)^u (-i\partial_R)^v \varphi_\beta(R,t) |I_{\alpha_i}\rangle = \left( E_0 - \frac{Q^2}{4m} \right)^u \mathbf{Q}^v D_{\alpha_o\alpha}(E_0,Q) D_{\beta\alpha_i}(E_0,Q), \tag{S25}$$

where $E_0$ is the total energy. Notice that, if $v$ is an odd number, the corresponding contact is a vector.

## SIV. MOMENTUM TAIL

Theoretically, Operator Product Expansion (OPE) is an ideal tool to explore such universal physics [15, 16]. One can expand the product of two operators as

$$\mathcal{O}_i(R+x)\mathcal{O}_j(R)|_{x\to 0} = \sum_n C_{ij}^k(x)\mathcal{O}_k(R), \tag{S26}$$

where $\{\mathcal{O}_i\}$ is a set of local operators and $C_{ij}^k(x)$ are expansion functions. $C_{ij}^k(x)$ can be determined by calculating the matrix elements of the operators on both sides of Eq. (S26) in the two-body state $|Q/2+k,\sigma; Q/2-k,\sigma'\rangle$. After the Fourier transform, this gives the major contribution at large momentum. There is a similar expansion in time direction.

By using the Fourier transformation on both sides of Eq. (S26), we have the expression of momentum distribution as [16]

$$n_{\sigma'\sigma}(q) = \int \frac{dR}{L} \int dx\; e^{-iqx} \left\langle \psi_\sigma^\dagger(R+x)\psi_{\sigma'}(R) \right\rangle, \tag{S27}$$

where $q$ is the relative momentum. This correspond to consider $\mathcal{O}_i = \psi_\sigma^\dagger$ and $\mathcal{O}_j = \psi_{\sigma'}$ in (S26).

Physically, we know that SOC should indeed make spin $\uparrow$ and $\downarrow$ different. Hence we consider the momentum distribution matrix $n_{\sigma'\sigma}(q) = \langle a_{q,\sigma}^\dagger a_{q,\sigma'}\rangle$, where $n_{\sigma'\sigma}(q)$ is a $2\times 2$ matrix in spin space.

There are four types of diagrams which can be used to denote the operators on the left-hand side of OPE equation (S26). However, the only nonanalyticity comes from the diagram as shown in Fig. S3. Therefore, with the Fourier transforms, we get the momentum distribution matrix as (the derivations are given in the Appendix)

$$n(q) = \sum_{\alpha,\beta=S,P} (-i)^2 D_{\alpha_o\alpha}(E_0,Q) D_{\beta\alpha_i}(E_0,Q) \int_{-\infty}^{\infty} \frac{dp_0}{2\pi} q^{l_\alpha+l_\beta} G(E_0-p_0,q)\sigma_\beta G^T(p_0,Q-q)\sigma_\alpha^\dagger G(E_0-p_0,q), \tag{S28}$$

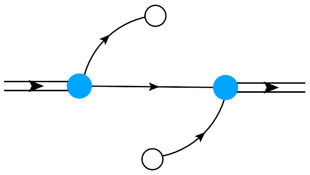

FIG. S3. (Color online) Feynman diagram for the matrix elements of the operator $\psi_\sigma^\dagger(R+x)\psi_{\sigma'}(R)$.

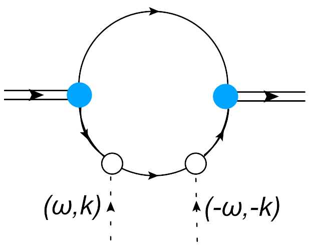


FIG. S4. (Color online) Feynman diagram for the matrix element of $\int dt\ e^{i\omega t} \int dx\ e^{-ikx} \mathcal{T} \mathcal{O}_{\sigma 3}(R+x,t)\mathcal{O}^\dagger_{\sigma' 3}(R,0)$ ($\sigma =\uparrow,\downarrow$).

where $E_0 = Q^2/(4m) + k^2/m$ is the total energy, $Q$ is the total momentum.

Keeping every element up to the first order with $u = v = 0$ and matching with Eq. (S25), we have the momentum distribution matrix:

$$n(q) \sim \begin{pmatrix} \frac{C_{PP}}{q^2L} + \frac{2\hat{\mathbf{q}}\cdot\mathbf{C}_{Q1}}{q^3L} + \frac{2C_r - 2k_0^2 C_{PP} - 2k_0\hat{\mathbf{q}}\cdot\mathbf{C}_{Q1} + 5C_{Q2}/2}{q^4L} + \frac{C_{SS}}{q^4L} & -\frac{C_{SP}}{q^3L} - \frac{2k_0C_{SP} + 2\hat{\mathbf{q}}\cdot\mathbf{C}_{SPQ1}}{q^4L} - \frac{m\Omega C_{PP}}{q^4L} \\ -\frac{C_{PS}}{q^3L} - \frac{2k_0C_{PS} + 2\hat{\mathbf{q}}\cdot\mathbf{C}_{PSQ1}}{q^4L} - \frac{m\Omega C_{PP}}{q^4L} & \frac{C_{SS}}{q^4L} \end{pmatrix}, \tag{S29}$$

where $\hat{\mathbf{q}}$ is the unit vector, we use $C_{PP} = C_{PP}^{(0,0)}$, $\mathbf{C}_{Q1} = C_{PP}^{(0,1)}$, $C_r = C_{PP}^{(1,0)}$, $C_{Q2} = C_{PP}^{(0,2)}$, $C_{PS} = C_{PS}^{(0,0)}$, $C_{SP} = C_{SP}^{(0,0)}$, $\mathbf{C}_{PSQ1} = C_{PS}^{(0,1)}$, $\mathbf{C}_{SPQ1} = C_{SP}^{(0,1)}$, and $C_{SS} = C_{SS}^{(0,0)}$. Note that $u = v = 0$ means the momentum distribution matrix does not receive contribution from momentum shift. If one wants to shift the momentum, the momentum of $p$-wave dimer also shift and different terms with $(u \neq 0, v \neq 0)$ would mix.

## SV. RAMAN SPECTROSCOPY

The Raman spectroscopy can be used as an important experimental tool in cold atom systems. When the transfer momentum and frequency is larger compared to the many-body scale, the Raman spectroscopy can be related to the contacts.

Consider we apply a Raman coupling with frequency $\omega$ and momentum $k$ is applied to transfers fermions from the internal spin state $|\sigma\rangle$ ($\sigma =\uparrow,\downarrow$) into a third spin state $|3\rangle$. The Hamiltonian reads

$$H_c = \sum_\sigma \Omega_\sigma \int dx\ e^{i(kx-\omega t)} \mathcal{O}_{\sigma 3}(x,t) + \text{H.c.}, \tag{S30}$$

where $\mathcal{O}_{\sigma 3}(x,t) \equiv \psi_3^\dagger(x,t)\psi_\sigma(x,t)$, $\Omega_\sigma$ is the radio frequency Rabi frequency determined by the strength of the radio frequency signal, and we assume $\omega > 0$.

The transition rate function $R(\omega,k)$ is given by the Fermi golden rule, which is related to the imaginary part of the time-ordered two-point correlation function [17, 18]

$$\Gamma^R_{\sigma\sigma'}(\omega,k) = \frac{1}{\pi}\text{Im} \int dR \int dt\ e^{i\omega t} \int dx\ e^{-ikx} i \left\langle \mathcal{T}\mathcal{O}_{\sigma 3}(R+x,t)\mathcal{O}^\dagger_{\sigma' 3}(R,0) \right\rangle, \tag{S31}$$

where $\mathcal{T}$ is the time-ordering operator. Explicitly, we have the transition rate function $R(\omega,k)$

$$R(\omega,k) = 2\pi \sum_{\sigma\sigma'} \Omega_\sigma \Omega^*_{\sigma'} \Gamma^R_{\sigma\sigma'}(\omega,k). \tag{S32}$$

We can evaluate the diagram in Figs. S4 as (the derivations are given in the Appendix)

$$\Gamma^R_{\sigma\sigma'}(\omega,k) = \frac{1}{\pi}\mathrm{Im}\; i \sum_{\alpha,\beta=S,P}(-i)^2 D_{\alpha_o\alpha}(E_0,Q)D_{\beta\alpha_i}(E_0,Q) \times \int \frac{dp dp_0}{(2\pi)^2} p^{l_\alpha+l_\beta} G_0(E_0-p_0+\omega,p+k) \times \left[G(E_0-p_0,p)\sigma^\dagger_\beta G^T(p_0,Q-p)\sigma_\alpha G(E_0-p_0,p)\right]_{\sigma\sigma'}, \tag{S33}$$

where $E_0 = Q^2/(4m) + q^2/m$ is the total energy, $Q$ is the total momentum, and we have defined $G_0(p_0,p) = i/(p_0 - p^2/(2m) + i0^+)$.

Matching Eq. (S31) with Eq. (S25), we have the Raman transfer rate from Eq. (S31) in high-frequency and large-momentum limit:

$$\Gamma^R(\omega,k) = \frac{2m}{\pi\sqrt{4m\omega-k^2}} \begin{pmatrix} \frac{2m\omega C_{PP}}{(k^2-2m\omega)^2} & \frac{k\left(k^2-6m\omega\right)C_{SP}}{(k^2-2m\omega)^3} \\ \frac{k\left(k^2-6m\omega\right)C_{PS}}{(k^2-2m\omega)^3} & \frac{2\left[4(m\omega)^2+4k^2m\omega-k^4\right]C_{SS}}{(k^2-2m\omega)^4} \end{pmatrix}. \tag{S34}$$

Here we have assumed $\omega > k^2/(4m)$. Taking the limit of $k=0$ leads to the high-frequency tail of the radio-frequency spectral $\Gamma^{rf}_{\sigma\sigma'}(\omega) = \Gamma^R_{\sigma\sigma'}(\omega,0)$. Therefore, we have

$$\Gamma^{rf}(\omega) = \frac{m}{2\pi} \begin{pmatrix} \frac{C_{PP}}{(m\omega)^{3/2}} & 0 \\ 0 & \frac{C_{SS}}{(m\omega)^{5/2}} \end{pmatrix}. \tag{S35}$$

## SVI. OTHER UNIVERSAL RELATIONS

### A. Adiabatic relations

The traditional $s$- and $p$-wave adiabatic relations are given by [4, 5]

$$\frac{C_{SS}}{2m} \equiv \frac{\partial E}{\partial a_s} = -\int dR \left\langle \frac{\partial \mathcal{L}(R)}{\partial a_s} \right\rangle = \frac{m}{2}\int dR \left\langle \varphi^\dagger_S(R)\varphi_S(R) \right\rangle, \tag{S36}$$

$$\frac{C_{PP}}{4m} \equiv -\frac{\partial E}{\partial a_p^{-1}} = \int dR \left\langle \frac{\partial \mathcal{L}(R)}{\partial a_p^{-1}} \right\rangle = \frac{m}{4}\int dR \left\langle \varphi^\dagger_P(R)\varphi_P(R) \right\rangle, \tag{S37}$$

where $E$ is the total energy of the many-body system, $\mathcal{L}(R)$ is the density of the Lagrangian (S23), $C_{SS}$ ($C_{PP}$) is the 1D $s(p)$-wave contact.

When SOC is present, there are two new parameters $k_0$ and $\Omega$. One can define two new contacts $C_\lambda$ and $C_\Omega$ as

$$C_\lambda \equiv -\int dR \left\langle \frac{\partial \mathcal{L}(R)}{\partial k_0} \right\rangle, \tag{S38}$$

$$C_\Omega \equiv -\int dR \left\langle \frac{\partial \mathcal{L}(R)}{\partial \Omega} \right\rangle. \tag{S39}$$

Here, $C_\lambda$ and $C_\Omega$ refer to only single-atom operators which give nonzero matrix elements in the single-atom sector. The momentum distribution under single-particle states is just a delta function, so that $C_\lambda$ and $C_\Omega$ will not contribute to the large-momentum tail, which is different from $C_{SS}$ and $C_{PP}$ [1]. However, both $k_0$ and $\Omega$ have nonzero energy scale, so that they would appear in the pressure relation and viral theorem.

### B. Pressure relation

For a uniform gas, the pressure relation can be derived following the expression of the Helmholtz free energy density $\mathcal{F} = F/L$ which can be expressed in terms of [4, 16, 19]

$$\mathcal{F}(T,n_\uparrow,n_\downarrow,a_s,a_p,k_0,\Omega) = \frac{k_F^3}{2m} f\left(\frac{2mT}{k_F^2}, \frac{n_\uparrow}{k_F}, \frac{n_\downarrow}{k_F}, a_s k_F, a_p k_F, \frac{k_0}{k_F}, \frac{2m\Omega}{k_F^2}\right), \tag{S40}$$

where $L$ is the length along the $x$ direction, $f$ is a dimensionless function, $T$ is the temperature, $n = n_\uparrow + n_\downarrow = k_F/\pi$ is the Fermi particle number density, and $k_F$ is the Fermi wave vector.

Equation (S40) implies the scaling behavior of the Helmholtz free energy density as follows:

$$\tilde{\lambda}^3 \mathcal{F}(T, n_\uparrow, n_\downarrow, a_s, a_p, k_0, \Omega) = \mathcal{F}\left(\tilde{\lambda}^2 T, \tilde{\lambda} n_\uparrow, \tilde{\lambda} n_\downarrow, \tilde{\lambda}^{-1} a_s, \tilde{\lambda}^{-1} a_p, \tilde{\lambda} k_0, \tilde{\lambda}^2 \Omega\right), \tag{S41}$$

where $\tilde{\lambda}$ is a dimensionless and arbitrary parameter.

Taking the derivative of Eq. (S41) with respect to $\tilde{\lambda}$ at $\tilde{\lambda} = 1$, we have

$$3\mathcal{F} = \left(2T\frac{\partial}{\partial T} + n_\uparrow \frac{\partial}{\partial n_\uparrow} + n_\downarrow \frac{\partial}{\partial n_\downarrow} - a_s \frac{\partial}{\partial a_s} - a_p \frac{\partial}{\partial a_p} + k_0 \frac{\partial}{\partial k_0} + 2\Omega \frac{\partial}{\partial \Omega}\right) \mathcal{F}. \tag{S42}$$

Replacing the free energy density $\mathcal{F}$ in the left side of Eq. (S42) by $n_\uparrow \mu_\uparrow + n_\downarrow \mu_\downarrow - \mathcal{P}$ and substituting $S = -\partial F/\partial T$ and $\mu_\sigma = \partial F/\partial n_\sigma$ into Eq. (S42), one gets

$$3(n_\uparrow \mu_\uparrow + n_\downarrow \mu_\downarrow - \mathcal{P}) = -2TS + n_\uparrow \mu_\uparrow + n_\downarrow \mu_\downarrow - a_s \frac{\partial \mathcal{F}}{\partial a_s} - a_p \frac{\partial \mathcal{F}}{\partial a_p} + k_0 \frac{\partial \mathcal{F}}{\partial k_0} + 2\Omega \frac{\partial \mathcal{F}}{\partial \Omega}, \tag{S43}$$

where $\mathcal{P}$ is the pressure density, $S$ is the entropy, and $\mu_\sigma$ is the chemical potentail with spin $\sigma$.

Using the adiabatic relations (S36), (S37), (S38) and (S39), we can get the pressure relation as

$$\mathcal{P} = 2\mathcal{E} + \frac{a_s C_{SS}}{2mL} + \frac{C_{PP}}{4ma_p L} - \frac{k_0 C_\lambda}{L} - \frac{2\Omega C_\Omega}{L}, \tag{S44}$$

where $\mathcal{E} = E/L$ is the energy density and we use $E = F + TS$ and

$$-a_p \frac{\partial E}{\partial a_p} = -a_p \frac{\partial E}{\partial a_p^{-1}} \frac{\partial a_p^{-1}}{\partial a_p} = -\frac{C_{PP}}{4ma_p}. \tag{S45}$$

### C. Virial theorem

For an atomic gas in a harmonic potential $V_T = m\omega^2 x^2/2$ with the trapping frequency $\omega$, the free energy can be expressed in terms of [4, 16, 19]

$$F(T, \omega, a_s, a_p, k_0, \Omega, N_\uparrow, N_\downarrow) = \omega \tilde{f}(T/\omega, \omega/\omega, a_s/a_{\rm ho}, a_p/a_{\rm ho}, k_0 a_{\rm ho}, \Omega/\omega, N_\uparrow, N_\downarrow), \tag{S46}$$

where $N = N_\uparrow + N_\downarrow$ is the particle number, $a_{\rm ho} = \sqrt{2/(m\omega)}$ is the harmonic oscillator length and the dimensionless function $\tilde{f}$ is dependent on the dimensionless ratios $T/\omega$, $a_s/a_{\rm ho}$, $a_p/a_{\rm ho}$, $k_0 a_{\rm ho}$, $\Omega/\omega$, and particle numbers $N_\uparrow$ and $N_\downarrow$.

With Eq. (S46), we can get the scaling law

$$\tilde{\lambda} F(T, \omega, a_s, a_p, k_0, \Omega, N_\uparrow, N_\downarrow) = F(\tilde{\lambda} T, \tilde{\lambda}\omega, \tilde{\lambda}^{-1/2} a_s, \tilde{\lambda}^{-1/2} a_p, \tilde{\lambda}^{1/2} k_0, \tilde{\lambda}\Omega, N_\uparrow, N_\downarrow), \tag{S47}$$

where $\tilde{\lambda}$ is a dimensionless and arbitrary parameter.

The derivative of Eq. (S47) with respect to $\tilde{\lambda}$ at $\tilde{\lambda} = 1$ gives

$$F = \left(T\frac{\partial}{\partial T} + \omega \frac{\partial}{\partial \omega} - \frac{1}{2} a_s \frac{\partial}{\partial a_s} - \frac{1}{2} a_p \frac{\partial}{\partial a_p} + \frac{1}{2} k_0 \frac{\partial}{\partial k_0} + \Omega \frac{\partial}{\partial \Omega}\right) F. \tag{S48}$$

Substituting $E = F + TS$ and $S = -\partial F/\partial T$ into Eq. (S48), one gets

$$E = \left(\omega \frac{\partial}{\partial \omega} - \frac{1}{2} a_s \frac{\partial}{\partial a_s} - \frac{1}{2} a_p \frac{\partial}{\partial a_p} + \frac{1}{2} k_0 \frac{\partial}{\partial k_0} + \Omega \frac{\partial}{\partial \Omega}\right) E, \tag{S49}$$

which, together with the Hellmann-Feynman theorem and the adiabatic relations (S36), (S37), (S38) and (S39), gives

$$E = 2\langle V_T \rangle - \frac{a_s C_{SS}}{4m} - \frac{C_{PP}}{8ma_p} + \frac{k_0 C_\lambda}{2} + \Omega C_\Omega. \tag{S50}$$

## SVII. CONTACTS IN TWO-BODY BOUND STATES

The inverse of the two-body $T$ matrix can be written as

$$T^{-1}(E_0,Q)\sim iD^{-1}(E_0,Q)=\begin{pmatrix} g_S^{-1}-i\Pi_{SS}(E_0,Q) & \delta_{SP}-i\Pi_{SP}(E_0,Q)\\ \delta_{PS}-i\Pi_{PS}(E_0,Q) & g_P^{-1}-i\Pi_{PP}(E_0,Q)\end{pmatrix}, \tag{S51}$$

where $\delta_{SP}=\delta_{PS}$ is a phenomenological parameter which is used to describe the bare coupling between $s$- and $p$-wave interactions on the two-body level. It corresponds to add a term $\sum_Q\left(\delta_{SP}\varphi^\dagger_{Q,S}\varphi_{Q,P}+\delta_{PS}\varphi^\dagger_{Q,P}\varphi_{Q,S}\right)$ in the Lagrangian. We introduce this additional coupling to derive the contact using the adiabatic relation.

The binding energy $E_b$ can be calculated by the pole of the $T$-matrix as $\det(T^{-1}(E_b,0))=0$, where $E_b=-\kappa^2/m$ with momentum $k=i\kappa$ [5]. We consider the case where $k_0$ and $\Omega$ can be treated perturbatively. To the $k_0^2$ and $\Omega$ order, we find

$$\begin{pmatrix} g_S^{-1}-i\Pi_{SS}(E_b,0) & \delta_{SP}-i\Pi_{SP}(E_b,0)\\ \delta_{PS}-i\Pi_{PS}(E_b,0) & g_P^{-1}-i\Pi_{PP}(E_b,0)\end{pmatrix}=\begin{pmatrix} -\frac{ma_s}{2}+\frac{m}{2\sqrt{-mE_b}} & \delta_{SP}+\frac{\sqrt{m}k_0\Omega}{8(-E_b)^{3/2}}\\ \delta_{SP}+\frac{\sqrt{m}k_0\Omega}{8(-E_b)^{3/2}} & \frac{m-a_pm\sqrt{-mE_b+k_0^2}}{4a_p}\end{pmatrix}, \tag{S52}$$

We assume $a_s>0$ and $a_p>0$. Without the coupling $\Omega$ and $\delta_{sp}$, the $s$- and $p$-wave dimers decouple. The binding energies are

$$E_b^{(s)}=-1/(ma_s^2),\qquad E_b^{(p)}=k_0^2/m-1/(ma_p^2). \tag{S53}$$

When $E_b^{(s)}$ and $E_b^{(p)}$ are almost degenrate, we expect strong mixing between the $s-$wave and the $p-$wave dimer. As a result, we expect a small off-diagonal term is important only when

$$1/(a_s^0)^2=1/(a_p^0)^2-k_0^2. \tag{S54}$$

we thus approximate the off-diagonal terms as $\delta_{SP}+\frac{k_0\Omega m^2(a_s^0)^3}{8}$. We further expand the diagonal terms near their own pole as

$$T^{-1}(E_b,0)\sim\begin{pmatrix} \frac{m^2a_s^3}{4}\left(E_b+\frac{1}{ma_s^2}\right) & \delta_{SP}+\frac{k_0\Omega m^2(a_s^0)^3}{8}\\ \delta_{SP}+\frac{k_0\Omega m^2(a_s^0)^3}{8} & \frac{m^2a_p}{8}\left(E_b+\frac{1}{ma_p^2}-\frac{k_0^2}{m}\right)\end{pmatrix}. \tag{S55}$$

Therefore, the pole of the $T$-matrix as $\det(T^{-1}(E_b,0))=0$ gives:

$$\begin{aligned}E_b^{(\pm)}=&-\frac{1}{2a_p^2a_s^2m^2}\left\{\left[a_s^2+a_p^2(1-a_s^2k_0^2)\right]m\right.\\ &\left.\pm\sqrt{a_s^4m^2+a_p^4m^2(1+a_s^2k_0^2)^2-2a_p^2a_s^2m^2(1+a_s^2k_0^2)+2a_p^3a_s[8\delta_{SP}+(a_s^0)^3k_0\Omega m^2]^2}\right\}.\end{aligned} \tag{S56}$$

The explicit formula for all contacts are given in the supplementary material. A plot for $E_b^{(\pm)}$ and contacts for $E_b^{(-)}$ are shown in Fig. S5 (a) and (c). Away from the degenerate point, $E_b^{(\pm)}$ approaches $E_b^{(s)}$ or $E_b^{(p)}$. Comparing Fig. S5 (a) with (c), it is found that the SOC parameters can open a gap between the two banding energies $E_b^{(+)}$ and $E_b^{(-)}$.

Further, with the adiabatic relations (S36), (S37), we can get the two-body contacts as

$$C_{SS}\equiv 2m\frac{\partial E_b^{(-)}}{\partial a_s}=\frac{2}{a_s^3}+\frac{-2a_s^2+2a_p^2(1+a_s^2k_0^2)+3a_pa_s(a_s^0)^6k_0^2m^2\Omega^2}{a_s^2\sqrt{a_s^2\{[a_s^2-a_p^2(1+a_s^2k_0^2)]^2+2a_p^3a_s(a_s^0)^6k_0^2m^2\Omega^2\}}}, \tag{S57}$$

$$C_{PP}\equiv -4m\frac{\partial E_b^{(-)}}{\partial a_p^{-1}}=\frac{4}{a_p}+\frac{2\{a_s[2a_s^2-2a_p^2(1+a_s^2k_0^2)]+a_p^3(a_s^0)^6k_0^2m^2\Omega^2\}}{a_pa_s\sqrt{[a_s^2-a_p^2(1+a_s^2k_0^2)]^2+2a_p^3a_s(a_s^0)^6k_0^2m^2\Omega^2}}, \tag{S58}$$

$$C_{SP}=C_{PS}\equiv -2m^2\frac{\partial E_b^{(-)}}{\partial\delta_{SP}}\bigg|_{\delta_{SP}=0}=\frac{16a_p(a_s^0)^3k_0m\Omega}{a_s\sqrt{[a_s^2-a_p^2(1+a_s^2k_0^2)]^2+2a_p^3a_s(a_s^0)^6k_0^2m^2\Omega^2}}, \tag{S59}$$

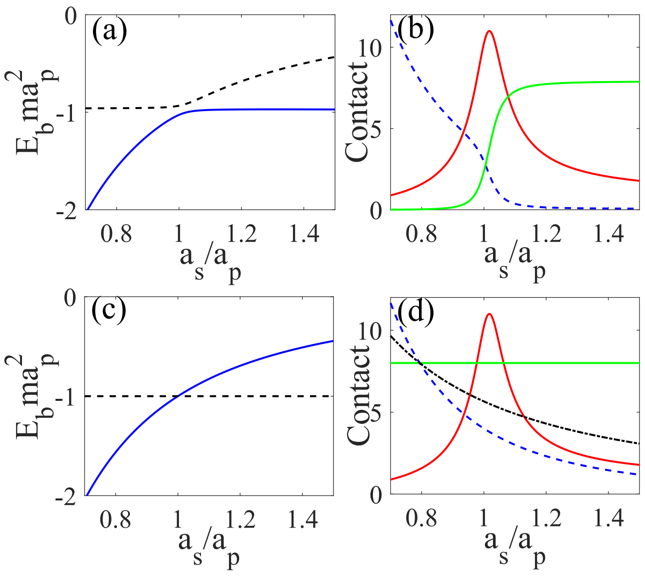


FIG. S5. (a) Dimensionless two-body banding energy versus $a_s/a_p$ with SOC. The black dashed curve denotes $E_b^{(+)}ma_p^2$ and the blue solid curve denotes $E_b^{(-)}ma_p^2$. (b) Dimensionless two-body contacts versus $a_s/a_p$ with SOC. (c) Dimensionless two-body banding energy versus $a_s/a_p$ without SOC. The black dashed curve denotes $E_b^{(p)}ma_p^2$ and the blue solid curve denotes $E_b^{(s)}ma_p^2$. (d) Dimensionless two-body contacts versus $a_s/a_p$ without SOC. As a comparsion, we also plot the $C_{SP}$ with finite SOC (the same curve as (b)). The red solid curve denotes $C_{SP}a_p^2$, the blue dashed curve denotes $C_{SS}a_p^3$, the green solid curve denotes $C_{PP}a_p$, and the black DotDashed curve denotes $\sqrt{C_{SS}C_{PP}}a_p^2$. Here, we choose the SOC parameters as $k_0a_p = 0.2$ and $m\Omega a_p^2 = 0.3$.

where we use $\delta_{SP} = 0$, $a_s^0 = a_s$, and $E_b^{(-)}$ to calculate the contacts as shown in Fig. S5(b). Consequently, for the diagonal components of the contact matrix, we have $C_{SS} \approx 0$ for $a_s/a_p \gg 1$ and $C_{PP} \approx 0$ for $a_s/a_p \ll 1$. Near the degenerate point $a_s/a_p \sim 1$, we see a peak for $C_{SP}$, indicating a large mixing between $s$- and $p-$wave dimers as expected.

Without SOC, one can have

$$C_{SS} \equiv 2m\frac{\partial E_b^{(s)}}{\partial a_s} = \frac{4}{a_s^3}, \tag{S60}$$

$$C_{PP} \equiv -4m\frac{\partial E_b^{(p)}}{\partial a_p^{-1}} = \frac{8}{a_p}, \tag{S61}$$

$$C_{SP} = C_{PS} = 0. \tag{S62}$$

Moreover, we also calculate the amplitude of the hybridized new contacts compared to the $s$- and $p$-wave ones without SOC as shown in Fig. S5 (d) to give the possibility of the measurement.

## SVIII. APPENDIX

### A. Derivations of Eq. (S10)

The polarization bubble can be calculated by the diagram in Fig. S6 as

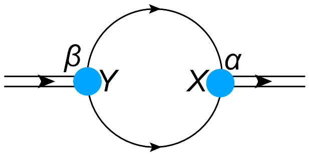


FIG. S6. Feynman diagram for the polarization bubble $\Pi_s$. Here, $X=(x_1,t_1)$ and $Y=(x_2,t_2)$.

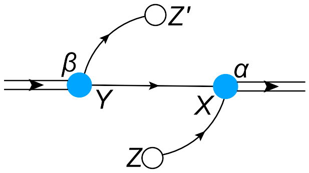


FIG. S7. Feynman diagram for the matrix of the operator $\Psi^{\dagger T}(Z)\Psi^{T}(Z')$. Here, $X=(x_1,t_1)$, $Y=(x_2,t_2)$, $Z=(x_3,t_3)$, and $Z'=(x_4,t_4)$.

$$\begin{aligned}
\Pi_{\alpha\beta}(E_0,Q) &= \int dXdY\ \mathrm{Tr}\left\langle \mathcal{T}\left[\frac{1}{2}\Psi^T(X)\sigma_\alpha\Psi(X)\right]\left[\frac{1}{2}\Psi^\dagger(Y)\sigma_\beta^\dagger\Psi^{\dagger T}(Y)\right]\right\rangle \\
&= \frac{1}{4}\int dXdY\ \mathrm{Tr}\left[\langle\mathcal{T}\Psi^T(X)\sigma_\alpha\Psi(X)\Psi^\dagger(Y)\sigma_\beta^\dagger\Psi^{\dagger T}(Y)\rangle + \langle\mathcal{T}\Psi^T(X)\sigma_\alpha\Psi(X)\Psi^\dagger(Y)\sigma_\beta^\dagger\Psi^{\dagger T}(Y)\rangle\right] \\
&= \frac{2}{4}\int dXdY\ \mathrm{Tr}\langle\mathcal{T}\Psi^T(X)\sigma_\alpha\Psi(X)\Psi^\dagger(Y)\sigma_\beta^\dagger\Psi^{\dagger T}(Y)\rangle\ (\textit{two equivalent contractions}), \\
&= \frac{1}{2}\int dXdY\ \mathrm{Tr}\left\langle\mathcal{T}\left[\Psi^T(X)\right]_{1a}(\sigma_\alpha)_{ab}\left[\Psi(X)\right]_{b1}\left[\Psi^\dagger(Y)\right]_{1m}\left(\sigma_\beta^\dagger\right)_{mn}\left[\Psi^{\dagger T}(Y)\right]_{n1}\right\rangle \\
&= \frac{1}{2}\int dXdY\ \mathrm{Tr}\left\langle\mathcal{T}\left[\Psi^T(X)\right]_{1a}\left[\Psi^{\dagger T}(Y)\right]_{n1}(\sigma_\alpha)_{ab}\left[\Psi(X)\right]_{b1}\left[\Psi^\dagger(Y)\right]_{1m}\left(\sigma_\beta^\dagger\right)_{mn}\right\rangle \\
&= \frac{1}{2}\int dXdY\ \mathrm{Tr}\left\langle\mathcal{T}\left[\Psi(X)\right]_{a1}\left[\Psi^\dagger(Y)\right]_{1n}\right\rangle(\sigma_\alpha)_{ab}\left[G(X-Y)\right]_{bm}\left(\sigma_\beta^\dagger\right)_{mn} \\
&= \frac{1}{2}\int dXdY\ \mathrm{Tr}\left[G(X-Y)\right]_{an}(\sigma_\alpha)_{ab}\left[G(X-Y)\right]_{bm}\left(\sigma_\beta^\dagger\right)_{mn} \\
&= \frac{1}{2}\int dXdY\ \mathrm{Tr}\left[G^T(X-Y)\right]_{na}(\sigma_\alpha)_{ab}\left[G(X-Y)\right]_{bm}\left(\sigma_\beta^\dagger\right)_{mn} \\
&= \int dXdY\ \frac{1}{2}\mathrm{Tr}\left[G^T(X-Y)\sigma_\alpha G(X-Y)\sigma_\beta^\dagger\right], \qquad \text{(S63)}
\end{aligned}$$

where $\int dXdY = \frac{1}{2}\int d(X+Y)d(X-Y)$, $\Psi = (\psi_\uparrow,\psi_\downarrow)^T$, $X=(x_1,t_1)$, $Y=(x_2,t_2)$, and we use the definition $G(X-Y)\equiv\langle\mathcal{T}\Psi(X)\Psi^\dagger(Y)\rangle$.

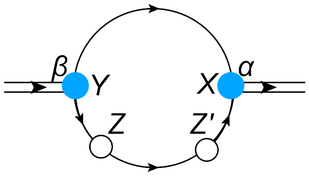


FIG. S8. (Color online) Feynman diagram for the matrix element of $\mathcal{O}_{\sigma 3}(R+x,t)\mathcal{O}^{\dagger}_{\sigma' 3}(R,0)$.

### B. Derivations of Eq. (S28)

As shown in Fig. S7, the vacuum expectation of the operator $\Psi^{\dagger T}(Z)\Psi^{T}(Z')$ is calculated as follows:

$$\left\langle O_{\alpha_o}\left|\Psi^{\dagger T}(Z)\Psi^{T}(Z')\right|I_{\alpha_i}\right\rangle = \begin{pmatrix} \left\langle O_{\alpha_o}\left|\psi^{\dagger}_{\uparrow}(Z)\psi_{\uparrow}(Z')\right|I_{\alpha_i}\right\rangle & \left\langle O_{\alpha_o}\left|\psi^{\dagger}_{\uparrow}(Z)\psi_{\downarrow}(Z')\right|I_{\alpha_i}\right\rangle \\ \left\langle O_{\alpha_o}\left|\psi^{\dagger}_{\downarrow}(Z)\psi_{\uparrow}(Z')\right|I_{\alpha_i}\right\rangle & \left\langle O_{\alpha_o}\left|\psi^{\dagger}_{\downarrow}(Z)\psi_{\downarrow}(Z')\right|I_{\alpha_i}\right\rangle \end{pmatrix}$$

$$= (-i)^2 D_{\alpha_o\alpha}(E_0,Q)D_{\beta\alpha_i}(E_0,Q)\int dXdY\ \left\langle \mathcal{T}\left[\frac{1}{2}\Psi^{T}(X)\sigma_\alpha\Psi(X)\right]\Psi^{\dagger T}(Z)\Psi^{T}(Z')\left[\frac{1}{2}\Psi^{\dagger}(Y)\sigma^{\dagger}_{\beta}\Psi^{\dagger T}(Y)\right]\right\rangle$$

$$= -\frac{D_{\alpha_o\alpha}(E_0,Q)D_{\beta\alpha_i}(E_0,Q)}{4}\int dXdY$$

$$\Big[\langle\mathcal{T}\Psi^{T}(X)\sigma_\alpha\Psi(X)\Psi^{\dagger T}(Z)\Psi^{T}(Z')\Psi^{\dagger}(Y)\sigma^{\dagger}_{\beta}\Psi^{\dagger T}(Y)\rangle + \langle\mathcal{T}\Psi^{T}(X)\sigma_\alpha\Psi(X)\Psi^{\dagger T}(Z)\Psi^{T}(Z')\Psi^{\dagger}(Y)\sigma^{\dagger}_{\beta}\Psi^{\dagger T}(Y)\rangle$$

$$+\langle\mathcal{T}\Psi^{T}(X)\sigma_\alpha\Psi(X)\Psi^{\dagger T}(Z)\Psi^{T}(Z')\Psi^{\dagger}(Y)\sigma^{\dagger}_{\beta}\Psi^{\dagger T}(Y)\rangle + \langle\mathcal{T}\Psi^{T}(X)\sigma_\alpha\Psi(X)\Psi^{\dagger T}(Z)\Psi^{T}(Z')\Psi^{\dagger}(Y)\sigma^{\dagger}_{\beta}\Psi^{\dagger T}(Y)\rangle\Big]$$

$$\sim \int dXdY\ \langle\mathcal{T}\Psi^{T}(X)\sigma_\alpha\Psi(X)\Psi^{\dagger T}(Z)\Psi^{T}(Z')\Psi^{\dagger}(Y)\sigma^{\dagger}_{\beta}\Psi^{\dagger T}(Y)\rangle\ (four\ equivalent\ contractions),$$

$$= \int dXdY\ \left\langle\mathcal{T}\left[\Psi^{T}(X)\right]_{1n}(\sigma_\alpha)_{nm}\left[\Psi(X)\right]_{m1}\left[\Psi^{\dagger T}(Z)\right]_{j1}\left[\Psi^{T}(Z')\right]_{1j}\left[\Psi^{\dagger}(Y)\right]_{1a}\left(\sigma^{\dagger}_{\beta}\right)_{ab}\left[\Psi^{\dagger T}(Y)\right]_{b1}\right\rangle$$

$$= \int dXdY\ \left\langle\mathcal{T}\left[\Psi(X)\right]_{n1}\left[\Psi^{\dagger}(Z)\right]_{1j}(\sigma_\alpha)_{nm}\left[\Psi(X)\right]_{m1}\left[\Psi^{\dagger}(Y)\right]_{1a}\left(\sigma^{\dagger}_{\beta}\right)_{ab}\left[\Psi(Z')\right]_{j1}\left[\Psi^{\dagger}(Y)\right]_{1b}\right\rangle$$

$$= \int dXdY\ \left[G(X-Z)\right]_{nj}(\sigma_\alpha)_{nm}\left[G(X-Y)\right]_{ma}\left(\sigma^{\dagger}_{\beta}\right)_{ab}\left[G(Z'-Y)\right]_{jb}$$

$$= \int dXdY\ \left[G^{T}(X-Z)\right]_{jn}(\sigma_\alpha)_{nm}\left[G(X-Y)\right]_{ma}\left(\sigma^{\dagger}_{\beta}\right)_{ab}\left[G^{T}(Z'-Y)\right]_{bj}$$

$$= \int dXdY\ G^{T}(X-Z)\sigma_\alpha G(X-Y)\sigma^{\dagger}_{\beta}G^{T}(Z'-Y), \tag{S64}$$

where $\int dXdY = \frac{1}{2}\int d(X+Y)d(X-Y)$, we label the field operator $\Psi = (\psi_\uparrow,\psi_\downarrow)^T$, $X=(x_1,t_1)$, $Y=(x_2,t_2)$, $Z=(x_3,t_3)$, $Z'=(x_4,t_4)$, and we use the definition $G(X-Y)\equiv\langle\mathcal{T}\Psi(X)\Psi^{\dagger}(Y)\rangle$.

Therefore, we have

$$\begin{pmatrix} \left\langle O_{\alpha_o}\left|\psi^{\dagger}_{\uparrow}(Z)\psi_{\uparrow}(Z')\right|I_{\alpha_i}\right\rangle & \left\langle O_{\alpha_o}\left|\psi^{\dagger}_{\uparrow}(Z)\psi_{\downarrow}(Z')\right|I_{s}\right\rangle \\ \left\langle O_{\alpha_o}\left|\psi^{\dagger}_{\downarrow}(Z)\psi_{\uparrow}(Z')\right|I_{\alpha_i}\right\rangle & \left\langle O_{\alpha_o}\left|\psi^{\dagger}_{\downarrow}(Z)\psi_{\downarrow}(Z')\right|I_{\alpha_i}\right\rangle \end{pmatrix}^{T} = \left[\left\langle O_{s}\left|\Psi^{\dagger T}(Z)\Psi^{T}(Z')\right|I_{\alpha_i}\right\rangle\right]^{T}$$

$$= -D_{\alpha_o\alpha}(E_0,Q)D_{\beta\alpha_i}(E_0,Q)\int dXdY\ G(Z'-Y)\sigma_\beta G^{T}(X-Y)\sigma^{\dagger}_{\alpha}G(X-Z), \tag{S65}$$

where we use $(ABCDE)^T = E^TD^TC^TB^TA^T$.

### C. Derivations of Eq. (S33)

Equation (S33) can be calculated by the diagram in Fig. S8 as

$$\begin{aligned}
&\left\langle O_{\alpha_o}\left|\mathcal{T}\mathcal{O}_{\sigma 3}(R+x,t)\mathcal{O}^{\dagger}_{\sigma' 3}(R,0)\right| I_{\alpha_i}\right\rangle\\
&\sim(-i)^2 D_{\alpha_o\alpha}(E_0,Q)D_{\beta\alpha_i}(E_0,Q)\int dXdY\ \left\langle\mathcal{T}\left[\frac{1}{2}\Psi^T(X)\sigma_\alpha\Psi(X)\right]\left[\Psi^\dagger(Z)\Psi(Z)\right]\left[\Psi^\dagger(Z')\Psi(Z')\right]\left[\frac{1}{2}\Psi^\dagger(Y)\sigma^\dagger_\beta\Psi^{\dagger T}(Y)\right]\right\rangle\\
&\sim\frac{1}{4}\int dXdY\left[\langle\mathcal{T}\Psi^T(X)\sigma_\alpha\Psi(X)\Psi^\dagger(Z)\Psi(Z)\Psi^\dagger(Z')\Psi(Z')\Psi^\dagger(Y)\sigma^\dagger_\beta\Psi^{\dagger T}(Y)\rangle\right.\\
&+\langle\mathcal{T}\Psi^T(X)\sigma_\alpha\Psi(X)\Psi^\dagger(Z)\Psi(Z)\Psi^\dagger(Z')\Psi(Z')\Psi^\dagger(Y)\sigma^\dagger_\beta\Psi^{\dagger T}(Y)\rangle\\
&+\langle\mathcal{T}\Psi^T(X)\sigma_\alpha\Psi(X)\Psi^\dagger(Z)\Psi(Z)\Psi^\dagger(Z')\Psi(Z')\Psi^\dagger(Y)\sigma^\dagger_\beta\Psi^{\dagger T}(Y)\rangle\\
&\left.+\langle\mathcal{T}\Psi^T(X)\sigma_\alpha\Psi(X)\Psi^\dagger(Z)\Psi(Z)\Psi^\dagger(Z')\Psi(Z')\Psi^\dagger(Y)\sigma^\dagger_\beta\Psi^{\dagger T}(Y)\rangle\right]\\
&=\int dXdY\ \langle\mathcal{T}\Psi^T(X)\sigma_\alpha\Psi(X)\Psi^\dagger(Z)\Psi(Z)\Psi^\dagger(Z')\Psi(Z')\Psi^\dagger(Y)\sigma^\dagger_\beta\Psi^{\dagger T}(Y)\rangle\ (\mathit{four\ equivalent\ contractions}),\\
&=\int dXdY\left\langle\mathcal{T}\left[\Psi^T(X)\right]_{1a}(\sigma_\alpha)_{ab}\left[\Psi(X)\right]_{b1}\left[\Psi^\dagger(Z)\right]_{1c}\left[\Psi(Z)\right]_{c1}\left[\Psi^\dagger(Z')\right]_{1d}\left[\Psi(Z')\right]_{d1}\left[\Psi^\dagger(Y)\right]_{1m}\left(\sigma^\dagger_\beta\right)_{mn}\left[\Psi^{\dagger T}(Y)\right]_{n1}\right\rangle\\
&=\int dXdY\left\langle\mathcal{T}\left[\Psi(X)\right]_{a1}(\sigma_\alpha)_{ab}\left[G(X-Z)\right]_{bc}\left[G(Z-Z')\right]_{cd}\left[G(Z'-Y)\right]_{dm}\left(\sigma^\dagger_\beta\right)_{mn}\left[\Psi^\dagger(Y)\right]_{1n}\right\rangle\\
&=\int dXdY\left\langle\mathcal{T}\left[\Psi(X)\right]_{a1}\left[\Psi^\dagger(Y)\right]_{1n}\right\rangle(\sigma_\alpha)_{ab}\left[G(X-Z)\right]_{bc}\left[G(Z-Z')\right]_{cd}\left[G(Z'-Y)\right]_{dm}\left(\sigma^\dagger_\beta\right)_{mn}\\
&=\int dXdY\ \ \left[G(X-Y)\right]_{an}(\sigma_\alpha)_{ab}\left[G(X-Z)\right]_{bc}\left[G(Z-Z')\right]_{cd}\left[G(Z'-Y)\right]_{dm}\left(\sigma^\dagger_\beta\right)_{mn}\\
&=\int dXdY\ \ \left[G^T(X-Y)\right]_{na}(\sigma_\alpha)_{ab}\left[G(X-Z)\right]_{bc}\left[G(Z-Z')\right]_{cd}\left[G(Z'-Y)\right]_{dm}\left(\sigma^\dagger_\beta\right)_{mn}\\
&=\int dXdY\ \ \left[G^T(X-Y)\sigma_\alpha G(X-Z)G(Z-Z')G(Z'-Y)\sigma^\dagger_\beta\right]\\
&\sim G_0(Z-Z')\int dXdY\ \ \left[G^T(X-Y)\sigma_\alpha G(X-Z)G(Z'-Y)\sigma^\dagger_\beta\right]\\
&=G_0(Z-Z')\int dXdY\ \ \left[G(Z'-Y)\sigma^\dagger_\beta G^T(X-Y)\sigma_\alpha G(X-Z)\right].
\end{aligned}\tag{S66}$$

### D. $T$ matrix for $s$ wave without SOC

As shown in Fig. S9(a), the two-body $T$ matrix for $s$ wave is given by [20]

$$-iT_s(E_0,Q)=\frac{-ig_S}{1-(-ig_S)\Pi_s(E_0,Q)}.\tag{S67}$$

As shown in Fig. S9(c), the dimer propagator matrix for $s$ wave is given by

$$D_{SS}(E_0,Q)=\frac{ig_S}{1-(ig_S)\Pi_{SS}(E_0,Q)},\tag{S68}$$

With $D_{SS}(E_0,Q)=iT_s(E_0,Q)$, one can get $\Pi_{SS}(E_0,Q)=-\Pi_s(E_0,Q)$.

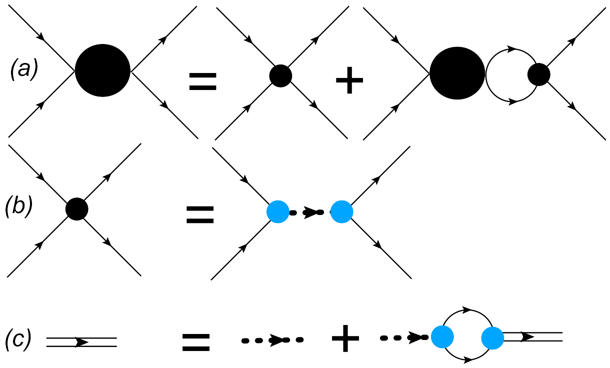


FIG. S9. (a) Diagrams for the $T$ matrix of $s$-wave without SOC. (b) Diagrams for the interaction vertex of $s$-wave. (c) Diagrams for the dimer propagator of $s$-wave. The black disk represents the $s$-wave $T$ matrix: $-iT_s$, the single line denotes the bare atom propagator $G$, the black dot represents the interaction vertex: $-ig_S$, the black dotted line denotes the bare dimer propagator $ig_S$, the double lines denote the dimer propagator $D$, and the blue dot represents the interaction vertex: $-i$.

### E. $T$ matrix for $p$ wave without SOC

The two-body $T$ matrix for $p$ wave is given by [20]

$$\frac{-iT_p(E_0,Q)}{qq'} = \frac{-ig_P}{1-(-ig_P)\Pi_p(E_0,Q)}. \tag{S69}$$

The dimer propagator matrix for $p$ wave is given by

$$D_{PP}(E_0,Q) = \frac{ig_P}{1-(ig_P)\Pi_{PP}(E_0,Q)}, \tag{S70}$$

With $D_{PP}(E_0,Q) = iT_p(E_0,Q)/(qq')$, one can get $\Pi_{PP}(E_0,Q) = -\Pi_p(E_0,Q)$.


[1] P. Zhang and N. Sun, "Universal relations for spin-orbit-coupled fermi gas near an $s$-wave resonance," Phys. Rev. A **97**, 040701 (2018).
[2] F. Qin, P. Zhang, and P.-L. Zhao, "Large-momentum tail of one-dimensional fermi gases with spin-orbit coupling," Phys. Rev. A **101**, 063619 (2020).
[3] M. Olshanii, "Atomic scattering in the presence of an external confinement and a gas of impenetrable bosons," Phys. Rev. Lett. **81**, 938 (1998).
[4] M. Barth and W. Zwerger, "Tan relations in one dimension," Annals of Physics **326**, 2544 (2011).
[5] X. Cui and H. Dong, "High-momentum distribution with a subleading $k^{-3}$ tail in odd-wave interacting one-dimensional fermi gases," Phys. Rev. A **94**, 063650 (2016).
[6] M. Olshanii, "Atomic scattering in the presence of an external confinement and a gas of impenetrable bosons," Phys. Rev. Lett. **81**, 938 (1998).
[7] T. Bergeman, M. G. Moore, and M. Olshanii, "Atom-atom scattering under cylindrical harmonic confinement: Numerical and analytic studies of the confinement induced resonance," Phys. Rev. Lett. **91**, 163201 (2003).
[8] X. Cui, "Quasi-one-dimensional atomic gases across wide and narrow confinement-induced resonances," Phys. Rev. A **86**, 012705 (2012).
[9] F. Qin, J.-S. Pan, S. Wang, and G.-C. Guo, "Width of the confinement-induced resonance in a quasi-one-dimensional trap with transverse anisotropy," The European Physical Journal D **71** (2017), 10.1140/epjd/e2017-80180-0.
[10] B. E. Granger and D. Blume, "Tuning the interactions of spin-polarized fermions using quasi-one-dimensional confinement," Phys. Rev. Lett. **92**, 133202 (2004).
[11] L. Pricoupenko, "Resonant scattering of ultracold atoms in low dimensions," Phys. Rev. Lett. **100**, 170404 (2008).
[12] S.-G. Peng, S. Tan, and K. Jiang, "Manipulation of $p$-wave scattering of cold atoms in low dimensions using the magnetic field vector," Phys. Rev. Lett. **112**, 250401 (2014).
[13] D. V. Kurlov and G. V. Shlyapnikov, "Two-body relaxation of spin-polarized fermions in reduced dimensionalities near a $p$-wave feshbach resonance," Phys. Rev. A **95**, 032710 (2017).
[14] Y.-T. Chang, R. Senaratne, D. Cavazos-Cavazos, and R. G. Hulet, "Collisional loss of one-dimensional fermions near a $p$-wave feshbach resonance," (2020), arXiv:2007.03723 [physics.atom-ph].

[15] E. Braaten and L. Platter, "Exact relations for a strongly interacting fermi gas from the operator product expansion," Phys. Rev. Lett. **100**, 205301 (2008).
[16] E. Braaten, D. Kang, and L. Platter, "Universal relations for a strongly interacting fermi gas near a feshbach resonance," Phys. Rev. A **78**, 053606 (2008).
[17] E. Braaten, D. Kang, and L. Platter, "Short-time operator product expansion for rf spectroscopy of a strongly interacting fermi gas," Phys. Rev. Lett. **104**, 223004 (2010).
[18] J. Hofmann, "Current response, structure factor and hydrodynamic quantities of a two- and three-dimensional fermi gas from the operator-product expansion," Phys. Rev. A **84**, 043603 (2011).
[19] X. Cui, "Universal one-dimensional atomic gases near odd-wave resonance," Phys. Rev. A **94**, 043636 (2016).
[20] V. Gurarie and L. Radzihovsky, "Resonantly paired fermionic superfluids," Annals of Physics **322**, 2 (2007), january Special Issue 2007.
